# Supplementary material for: Unsupervised Massive MIMO Channel Estimation with Dual-Path Knowledge-Aware Auto-Encoders
Source: arXiv:2305.18744 source file (2023-05-30)
Supplement: Supplementary file 1 [file temp.tex]

\section{Convergence of the Channel Estimation Network} \label{proof: Convergence of the Channel Estimation Network}

For the update of the channel estimation network, the estimation of the AoA {$\bm{\widehat{\theta}}$} can be seen as constant {$\bm{\overline{\theta}}$}. Ignoring interference between different users, the loss function can be written as:
\begin{equation} \label{eqn: loss function for channel estimation network}
    \begin{aligned}
            loss^{\left( \alpha, \phi \right)}   
                    =       &        
                \mathbb{E} \left[
                    \sum^{M-1}_{m=0} \sum^{K-1}_{k=0} \left( 
                        \alpha_{m,k}^2 + \widehat{\alpha}_{m,k}^2 
                        - 2\alpha_{m,k} \widehat{\alpha}_{m,k}
                        \right. \right. , \\
                            &   
                \left. \left.
                            \cos \left(
                                \left(\phi_{m,k} - \widehat{\phi}_{m,k} \right)
                                - \left(\bm{\Psi}\left(\theta_{k} \right) - \bm{\Psi}\left(\overline{\theta}_{k} \right) \right)
                            \right)
                    \right)
                \right].
    \end{aligned}
\end{equation}
Where the subscript {$m,k$} means the signal received at the {$m$}th snapshot from the {$k$}th users. {$\left[ \alpha, \phi, \theta \right]$} are the target parameters of path gain, path angle and AoA, respectively, while {$\left[ \widehat{\alpha}, \widehat{\phi}, \overline{\theta} \right]$} are the estimated of that.

Let 
$\eta = \left(
    \phi_{m,k} - \widehat{\phi}_{m,k} \right)
    - \left(\bm{\Psi}\left(\theta_{k} \right) - \bm{\Psi}\left(\overline{\theta}_{k} \right) \right)$
and $\alpha, \widehat{\alpha}$ regard as $\alpha_{m,k}, \widehat{\alpha}_{m,k}$.
\begin{equation}
    \left \{
        \begin{aligned}
            & 0 \leq 
            \left( \alpha - \widehat{\alpha} \right)^2 \leq
            \alpha^2 + \widehat{\alpha}^2 
                - 2\alpha \widehat{\alpha} \cos{\eta} &
            0 < \cos{\eta} \leq 1  \\
            & 0 < 
            \alpha^2 + \widehat{\alpha}^2 \leq
            \alpha^2 + \widehat{\alpha}^2 
                - 2\alpha \widehat{\alpha} \cos{\eta} &
            -1 \leq \cos{\eta} \leq 0
        \end{aligned}
    \right..
\end{equation}

According to \eqref{eqn: loss function for channel estimation network}, if $loss^{(\alpha, \phi)} \rightarrow 0$, where "$\rightarrow$" means "tend to", there are $\cos{\eta} \rightarrow 1$ and $\eta \rightarrow 2\pi l, l \in Z$. Thus, 
$\left[
    \left( \phi - \widehat{\phi} \right) 
    - \frac{2\pi(n-1)d}{\lambda} 
        \left( \sin{\theta} - \sin{\overline{\theta}} \right)
\right]
\rightarrow 2 \pi l, n = 1, 2,... ,N$

When it comes to the channel estimation network, the weight of the back propagation is only dependent on $\alpha$ and $\phi$. Assume that $\sin{\overline{\theta} \rightarrow} \sin{\theta}$, then $\widehat{\phi} - \phi \rightarrow 2\pi l$, which means $\widehat{\phi} \rightarrow \phi + 2\pi l$. For {$\phi, \widehat{\phi} \in (-\pi, \pi]$}, there is $\widehat{\phi} \rightarrow \phi$. Thus
\begin{equation}
    loss^{(\alpha, \phi)} = 
    \alpha^2 + \widehat{\alpha}^2 - 2\alpha \widehat{\alpha} \cos{\eta}
    \rightarrow
    \left( \alpha - \widehat{\alpha} \right)^2
    \geq
    0.
\end{equation}

Then, when $\sin{\widehat{\theta} \rightarrow} \sin{\theta}$ and $\widehat{\phi} \rightarrow \phi$, $loss^{(\alpha, \phi)} \rightarrow 0$ means $\widehat{\alpha} \rightarrow \alpha$.
